# Supplementary material for: de Sitter Entanglement and Conformal Description of the Cosmological Horizon
Source: arXiv:1911.06627 source file (2019-12-20)
Supplement: Supplementary file 1 [file AppendixA.tex]

% Bppendix B

\chapter{Derivation of Liouville action} % MBin Bppendix title
\label{App:A} % For referencing this Bppendix elsewhere, use \ref{BppendixB}

The bosonic string coupled to two-dimensional quantum gravity  \cite{Polyakov:1981rd, Polyakov:1987zb,  Distler:1988jt, Knizhnik:1988ak, gervais1985, GERVAIS198259, DHoker:1982aa, YONEYA1984111, DHoker:1982wmk, Gervais:1982nw, Gervais:1983ry} has a partition function of the form
\begin{align}
\mathcal Z = \int \frac{\mathcal D g \mathcal D_g X}{\text{vol Diff}} \exp \left\{-S_M [X; g] - \frac{\mu_0}{2\pi}\int d^2 \zeta \sqrt{g} \right\}~,
\end{align}
where $\mu_0$ is related to the cosmological constant and vol Diff corresponds to action of the group  of two-dimensional diffeomorphisms and the group of local Weyl rescalings. This due to the fact that the path integral of the action contains an enormous amount of overcounting configurations $[X; g]$ and $[X`; g`]$ that are just related by diffeomorphisms and weyl rescaling, therefore they both describe the same physics. Therefore we divide by this number. The action 
\begin{align}
S_M [X;g] = \frac{1}{4\pi\alpha'}\int d^2 \zeta \sqrt{g} g^{a b}\partial_a X_\mu \partial_b X^\mu~,
\end{align}
corresponds to the Polyakov action \cite{Polyakov:1981rd, Brink:1976sc, Deser:1976eh} posses $d$ scalar fields $X$ propagating on $g$. The measure $\mathcal D_g X$ by using the norm of the variation of the fields 
\begin{align}\label{Dmeasure}
\int \mathcal D_g \delta X \exp\{ - ||\delta X||^2_g\} := 1~,
\end{align}
with the norm as
\begin{align}
 ||\delta X||^2_g := \int d^2\zeta \sqrt{g} \delta X_\mu \delta X^\mu
\end{align}
the same fashion leads to the only possibility of the norm of the metric
\begin{align}\label{normg}
||\delta g||^2_g = \int d^2\zeta \sqrt{g}\left(g^{ac}g^{bd} + C g^{ab}g^{cd}\right)\delta g_{ab}\delta g_{cd}~,
\end{align}
with $C$ a non-negative constant. This can be used to find the measure of integration using explicit decomposition of the metric variation. 
\\

The matter action is unvariant under a Weyl transformation of the metric $g \rightarrow \exp\{\beta\}g[\tau]$, with $\tau$ parameters,  such that $S_M [X; g] = S_M [X; \exp\{\beta\}g]$, but not the metric measure \eqref{Dmeasure} 
\begin{align}
\mathcal D_{\exp\{\beta\}g} X = \exp\left\{\frac{d}{24\pi\alpha'}S_L[\beta, g]\right\} \mathcal D_g X~,
\end{align} 
where the $S_L$ action is the Liouville action presented in \autoref{Chp:Liouville}
\begin{align}
S_L[\beta; g] = \int d^2\zeta \sqrt{g}\left(\frac{1}{2}g^{ab}\partial_a \beta \partial_b \beta + \beta R + \mu \exp\{\beta\}\right)~.
\end{align}
Where the Ricci tensor in two dimensions satisfy the relation
\begin{align}
\frac{1}{4\pi}\int d^2\zeta \sqrt{g} R = 2 - 2g~,
\end{align}
with $g$ as the genus of the Riemann surface $\Sigma$. Under parametrization of the metric $g$ by a diffeomorphism $D$ and Weyl rescaling $\phi_0$ implies $D(g) = \exp\{\phi_0\}\hat g$. We can exchange the integration over metrics $g$ over vector fields $\xi$ that generate infinitesimal diffeomorphisms, which Jacobian can be represented over the fields $b$ and $c$ that are called ghosts \cite{Distler:1988jt}
\begin{align}
\mathcal D_g b \mathcal D_g c \exp\{-S_{gh}[b,c;g]\}~,
\end{align}
where the ghost action it is invariant under Weyl rescaling of the metric. The measure of the ghost fields varies under this rescaling as
\begin{align}
\mathcal D_{\exp\{\beta\}g} b \mathcal D_{\exp\{\beta\}g}c = \exp\left\{\frac{-26}{24\pi}S_L[\beta; g]\right\}\mathcal D_{g}b\mathcal D_{g}c~,
\end{align}
which coincides with the measure of the matter measure in the critical dimension $d = 26$. For $d\neq 26$, thus the partition function vary as 
\begin{align}
\mathcal Z = \int [d\tau] \mathcal D_g \phi_0 \mathcal D_g b \mathcal D_g c \mathcal D_g X~, \exp\left\{ - \left[S_M[X; g] + S_{gh}[b,c ;g] + \frac{\mu_0}{2\pi}\int d^2\zeta \sqrt{g}\right]\right\}~.
\end{align}
Where $[d\tau]$ is the measure of the integration over the parameters. The measure of the of the Weyl rescaling $\phi_0$ is induced by \eqref{normg} 
\begin{align}
||\delta\phi_0||^2_g = \int d^2\zeta \sqrt{g} (\delta\phi_0)^2 = \int d^2\zeta \sqrt{\hat g}\exp\{\phi_0\}(\delta \phi_0)^2~.
\end{align}
The measures can be shifted in order to they to be independent of  $\phi_0$, picking a Jacobian $J(\phi, \hat g)$
\begin{align}
\mathcal D_g\phi_0 \mathcal D_g b \mathcal D_g c \mathcal D_{\hat g} X = \mathcal D_{\hat g} \phi \mathcal D_{\hat g} b \mathcal D_{\hat g} c \mathcal D_{\hat g} X~J(\phi,\hat g)~,
\end{align}
which is given by the exponent of a renormalizable local action 
\begin{align}
J(\phi, \hat g) = \exp\{-S[\phi; \hat g])\}~.
\end{align}
The action that satisfy this and is diffeomorphism invariant has the exact form \eqref{Lact}
\begin{align}
S[\phi;\hat g] ={}& \frac{1}{8\pi}\int d^\zeta \sqrt{\hat g}\left( \hat g^{ab}\partial_a \phi \partial_b \phi - Q\phi\hat R + 4\mu \exp\{\alpha \phi\}\right) \nonumber \\ ={}& \frac{1}{2\pi}\int d^2 z \left[ \partial\phi \bar\partial \phi \sqrt{\hat g}\left(\mu\exp\{\alpha\beta\}- \frac{1}{4}Q\phi\hat R \right)\right]~.
\end{align}
As it is presented in \autoref{Chp:Liouville} the action must be invariant under \eqref{conftrn} which leads to obtain an equality matching the measures which allow us to identify the different central charges and ask to the theory to be anomaly free. The central charge for the $\phi$-system \cite{Seiberg:1990eb} it has been derived in \autoref{Chp:Liouville}
\begin{align}
c_\phi = 1 + 3Q^2~,
\end{align}
and asking for the total conformal anomaly to vanish implies
\begin{align}
Q = \sqrt{\frac{25-d}{3}}~,
\end{align}
which is real for $d\leq 25$.
