# Supplementary material for: de Sitter Entanglement and Conformal Description of the Cosmological Horizon
Source: arXiv:1911.06627 source file (2019-12-20)
Supplement: Supplementary file 5 [file AppendixTemplate.tex]

% Appendix Template

\chapter{Appendix Title Here} % Main appendix title

\label{AppendixX} % Change X to a consecutive letter; for referencing this appendix elsewhere, use \ref{AppendixX}

Write your Appendix content here.
